# Supplementary material for: Chaotic stochastic resonance in Mackey-Glass equations
Source: arXiv:2505.04874 source file (2026-01-08)
Supplement: Supplementary file 1 [file Supplemental.pdf]

# Supplemental Material for “Coexistence of stochastic resonance and stochastic chaos in Mackey–Glass Equations”

Eiki Kojima<sup>1</sup> and Yuzuru Sato<sup>1,2,3</sup>

<sup>1</sup>*Department of Mathematics, Hokkaido University,  
N12 W7 Kita-ku, Sapporo, 0600812 Hokkaido, Japan*

<sup>2</sup>*RIES-MSU, Hokkaido University, N12 W7 Kita-ku, Sapporo, 0600812 Hokkaido, Japan*

<sup>3</sup>*London Mathematical Laboratory, 14 Buckingham Street, London WC2N 6DF, United Kingdom  
(Dated: July 17, 2025)*

## RANDOM PULLBACK ATTRACTOR AND RANDOM LYAPUNOV EXPONENT

To parametrize a noise realization  $\omega \in \Omega$  in time  $t$ , we introduce a family of measure-preserving maps  $\theta_t : \Omega \rightarrow \Omega$  satisfied with  $\theta_0 = \text{id}_\Omega$  and  $\theta_{s+t} = \theta_s \circ \theta_t$  for each time  $t$ . The time evolution of random dynamical systems can be described by the stochastic flow  $\Phi(t, \omega) : X \rightarrow X$  satisfied with the cocycle property  $\Phi(t+s, \omega) = \Phi(t, \theta_s(\omega)) \circ \Phi(s, \omega)$ . In the case of single attractor systems, a set  $\mathcal{A}(\omega)$  is called a random pullback attractor if it satisfies the three following conditions (see [1, 2] for the exact definition):

- i.  $\mathcal{A}(\omega)$  is a compact, i.e.,  $A(\omega) := \{x \in X \mid (\omega, x) \in \mathcal{A}(\omega)\} \subset X$  is compact for almost all  $\omega \in \Omega$ .
- ii.  $\mathcal{A}(\omega)$  is  $\Phi$ -invariant, i.e., for all  $t$ ,  $\Phi(t, \omega)A(\omega) = A(\theta_t \omega)$  for almost all  $\omega \in \Omega$ .
- iii.  $\mathcal{A}(\omega)$  is pullback attracting, i.e.,  $\lim_{t \rightarrow \infty} d_X(\Phi(t, \theta_{-t} \omega)B, A(\omega)) = 0$  holds for all  $B \subset X$  and for almost all  $\omega \in \Omega$ .

where  $d_X$  is the Hausdorff semi-distance.

A realization  $A(\omega)$  of a random pullback attractor  $\mathcal{A}(\omega)$  is approximated by a snapshot of trajectories evolving from a set of initial values  $B$ , with a fixed noise realization  $\omega$ , and with a integration period given by the pullback time  $t_p$ . For a precise numerical computation, a large number of initial points for  $B$  and a large pullback time  $t_p$  are adopted. The Lyapunov exponent of stochastic dynamics on random pullback attractors is given by the average expansion rate of perturbations, similarly to those of deterministic dynamics. For example, the Lyapunov exponent of a one-dimensional stochastic differential equation  $dx = f(x)dt + \sigma dW_t$ , where  $W_t$  is the Wiener process, is given by

$$\lambda(\omega, x_0) = \lim_{T \rightarrow \infty} \frac{1}{T} \int_0^T f'(\Phi(t, \omega)x_0)dt, \quad (\text{S.1})$$

where  $\Phi$  represents the stochastic flow, and  $x_0 \in X$  is the initial condition. Note that the Lyapunov exponent is a random variable in general. When the system is ergodic and has a single attractor,  $\lambda(\omega, x_0)$  is a constant for almost all  $\omega$  and for all  $x_0$ .

## BIFURCATION DIAGRAM OF RANDOM PULLBACK ATTRACTOR

We introduce a bifurcation diagram of pullback attractors for the stochastic Mackey–Glass equation (SMG). Plotting trajectories starting from many initial conditions with a fixed noise realization for each parameter, the bifurcation of random pullback attractors is successfully visualized. Similarly to random pullback attractors, this bifurcation diagram also evolves in time. In FIG. S1, emergence of the pseudo-periodic motion of the measure of all possible trajectories  $\rho_t$  is observed near  $a = 0.14$  and  $\sigma = 0.15$ .

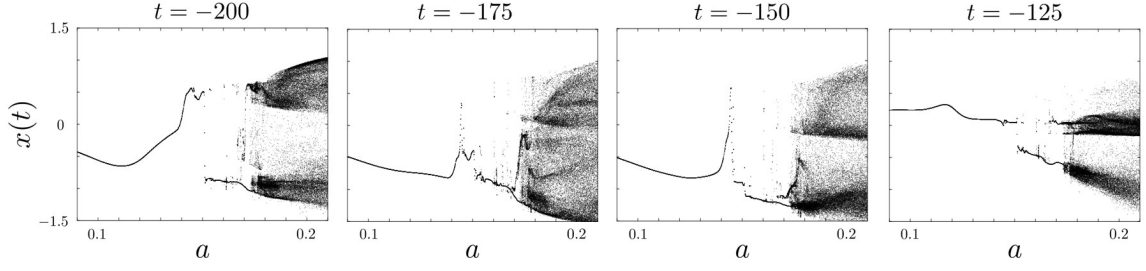

FIG. S1. Four snapshots of bifurcation diagrams of random pullback attractors with a fixed noise realization with  $\sigma = 0.15$ . For all values of  $a$ , random pullback attractors are computed using a fixed noise realization. The computation scheme is the same as that of FIG. 1 in the main text.

### LINEAR MODE ANALYSIS FOR THE UNSTABLE SPIRAL AT THE ORIGIN

When the delay  $\tau$  is sufficiently large, the peaks of the power spectra of the Mackey–Glass equation (MG) agree with the linear modes around fixed points [3]. The characteristic equations at fixed points  $x = 0, \pm x^*$ , where  $x^* = (\frac{a-b}{b})^{1/c}$

$$\begin{aligned} \chi + b - ae^{-\chi\tau} &= 0 & (x = 0), \\ \chi + b - (\frac{cb^2}{a} - (c-1)b)e^{-\chi\tau} &= 0 & (x = \pm x^*), \end{aligned} \quad (\text{S.2})$$

have an infinite number of roots  $\chi = \lambda_n, \mu_n$  ( $n = 0, \pm 1 \pm 2, \dots$ ) given by

$$\begin{aligned} \lambda_n &= -b + \frac{1}{\tau} W_n[a\tau \exp(b\tau)] & (x = 0), \\ \mu_n &= -b + \frac{1}{\tau} W_n\left[\left(\frac{cb^2}{a} - (c-1)b\right)\tau \exp(b\tau)\right] & (x = \pm x^*), \end{aligned} \quad (\text{S.3})$$

where  $W_n(z)$  is the Lambert W-function [4]. Using the asymptotic expansion of the Lambert W-function [5], the frequencies of linear modes around the fixed points are given by the imaginary part of  $\lambda_n, \mu_n$ , respectively expressed as

$$\begin{aligned} s_{2n} &:= \frac{1}{2\pi} \text{Im}(\lambda_n) \simeq \frac{2n}{2\tau} \left[ 1 - \frac{1}{b\tau + \ln(a\tau)} \right] & (x = 0), \\ s_{2n+1} &:= \frac{1}{2\pi} \text{Im}(\mu_n) = \frac{2n+1}{2\tau} \left[ 1 - \frac{1}{b\tau + \ln(\frac{cb^2}{a} - (c-1)b\tau)} \right] & (x = \pm x^*). \end{aligned} \quad (\text{S.4})$$

The even modes  $s_{2n}$  represent an unstable spiral around the origin, and the odd modes  $s_{2n+1}$  represent spirals around the fixed point  $x = \pm x^*$ . The characteristic frequencies of the dynamics dominated by odd modes at  $x = \pm x^*$  (FIG. S2). Adding the optimal noise, the odd modes are suppressed and the even modes become dominant, causing the emergence of stochastic resonance (SR) with resonant frequencies corresponding to the even mode.

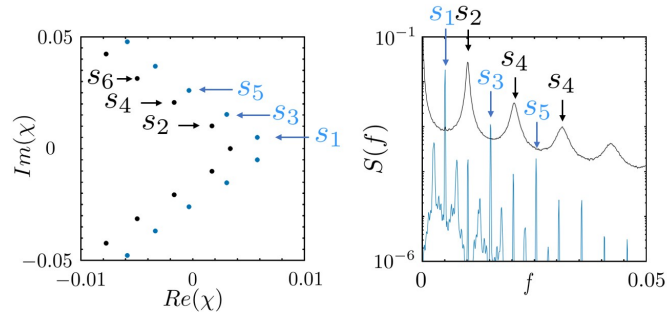

FIG. S2. Roots of linear modes  $\chi = \lambda_n, \mu_n$  are shown in the left panel. Black and blue points represent the linear modes at  $x = 0, \pm x^*$ , respectively. The power spectrum with  $\sigma = 0$  (blue line) and optimal noise  $\sigma = \sigma^*$  (black line) are shown in the right panel.

# STOCHASTIC RESONANCE WITH POINT, PERIODIC, AND STRANGE ATTRACTORS

In the weak nonlinearity region, adding noise to point, periodic, and strange attractors in MG with  $a = 0.12, 0.126, 0.14$ , SR switching between these attractors emerges. These SR occur in the same manner (FIG. S3), as each attractor becomes a random point attractor with negative Lyapunov exponents.

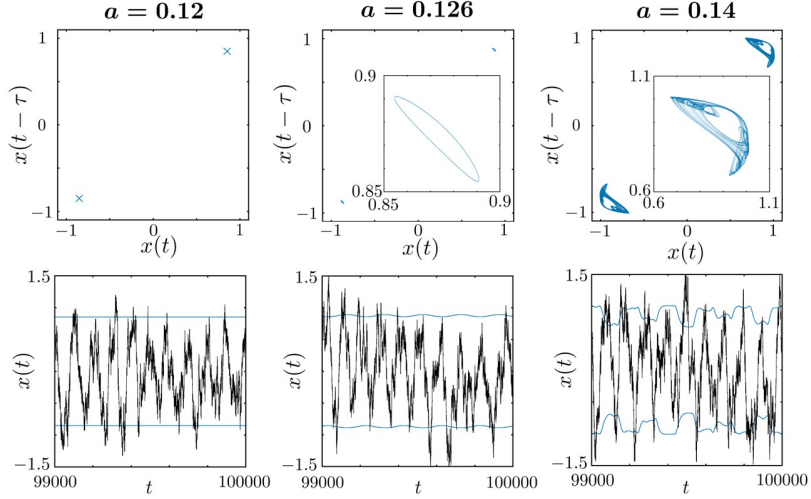

FIG. S3. Deterministic point, periodic, and strange attractors in the Mackey–Glass equation (MG) with  $a = 0.12, 0.126, 0.14$  are shown in the top panel. The inset shows a magnified view of the attractor. Time series at the deterministic case  $\sigma = 0$  (blue dots) and resonance case  $\sigma = \sigma^*$  (black dots) are shown in the bottom panel.

The power spectrum  $S(f)$  shows the harmonics under the optimal noise intensity  $\sigma = \sigma^*$ , and both  $S(f_1^*)$  and  $\lambda_1$  are maximized locally at  $\sigma = \sigma^*$ , exhibiting SR for  $a = 0.12, 0.126$ , and  $0.14$  (FIG. S4).

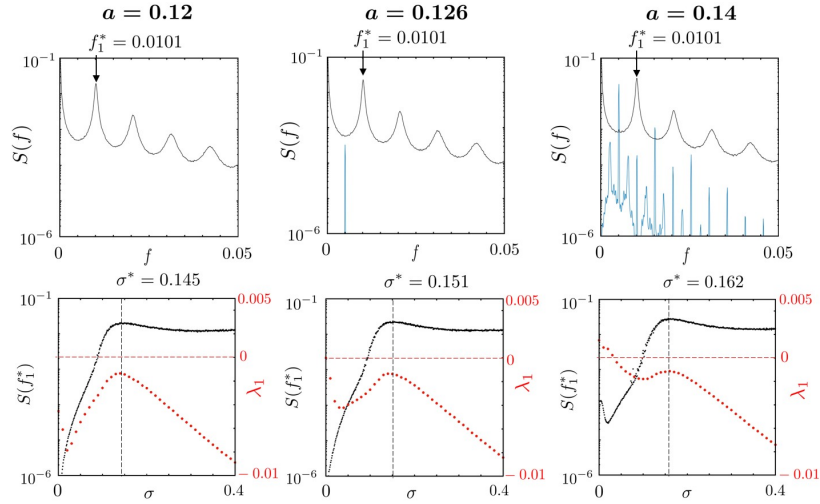

FIG. S4. Power spectra with  $\sigma = 0$  (blue lines) and optimal noise  $\sigma = \sigma^*$  (black lines) are shown in the top panel. The power of the main resonance frequency  $f_1^*$  (black points) and the largest Lyapunov exponent  $\lambda_1$  (red points) as a function of  $\sigma$  are shown in the bottom panel.

## SPACE-TIME REPRESENTATION

Trajectories of time delayed systems can be represented in a two-dimensional space-time diagram, introducing new coordinates  $t = n\tau + s$ ,  $n \in \mathbb{Z}$ ,  $s \in [0, \tau)$ . The diagram is constructed by splitting the time series of  $x(t)$  into segments  $X_n(s) = \{x(t) | (n-1)\tau \leq t < n\tau\}$  of length  $\tau$ , and representing them sequentially in  $n$ , where  $n$  is the time step, and  $s(0 \leq s < \tau)$  is the location in the memory space in each segment. The representation allows us to identify visually regular and irregular motion of the dynamics in the segments (FIG. S5 ).

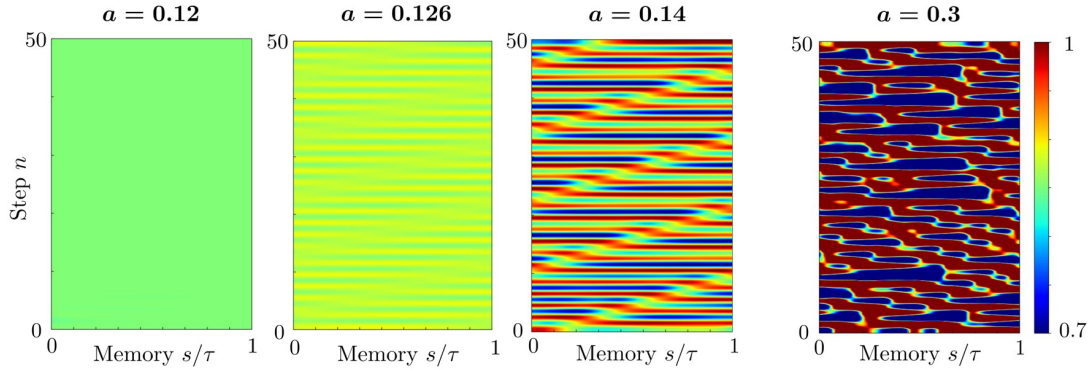

FIG. S5. Space-time representations of the MG for  $a = 0.12$  (fixed point),  $a = 0.126$  (limit cycle),  $a = 0.14$  (chaos), and  $a = 0.3$  (high-dimensional chaos).

These representations can be introduced for noised dynamics of SMG as well. In FIG. S6, the red and blue areas represent metastable states near the deterministic attractor. The SR and the chaotic SR with period  $T = \tau(1 + \epsilon)$  are observed as traveling waves. Notably, the chaotic SR (FIG. S6, right) exhibits stronger periodicity than the SR (FIG. S6, left 3 panels). Moreover, the chaotic structure inside the traveling waves is distinctly visible in the space-time representation, indicating the coexistence of SR and high-dimensional stochastic chaos.

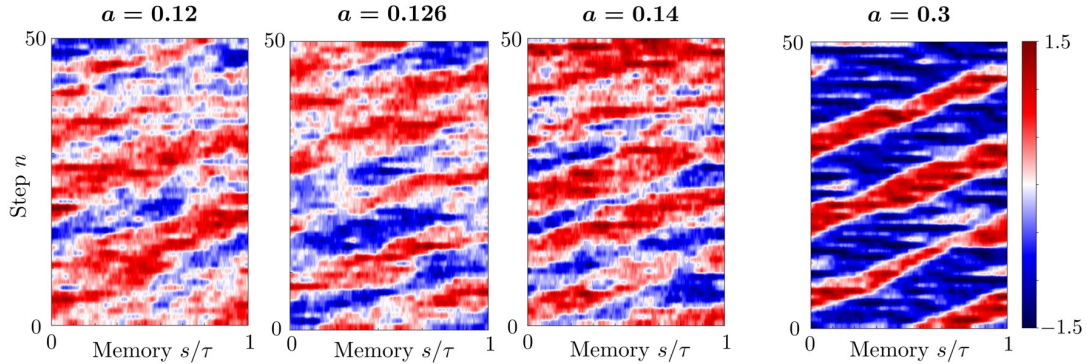

FIG. S6. Space-time representations of the stochastic Mackey–Glass equation (SMG) at the resonance point for  $a = 0.12$  (fixed point,  $\sigma^* = 0.145$ ),  $a = 0.126$  (limit cycle,  $\sigma^* = 0.151$ ),  $a = 0.14$  (chaos,  $\sigma^* = 0.162$ ), and  $a = 0.3$  (high-dimensional chaos,  $\sigma^* = 0.105$ ).

- 
- [1] L. Arnold, *Random Dynamical Systems* (Springer Berlin, Heidelberg, 1998).
  - [2] M. D. Chekroun, E. Simonnet, and M. Ghil, *Physica D: Nonlinear Phenomena* **240**, 1685 (2011).
  - [3] B. Mensour and A. Longtin, *Physica D: Nonlinear Phenomena* **113**, 1 (1998).
  - [4] R. M. Corless, G. H. Gonnet, D. E. Hare, D. J. Jeffrey, and D. E. Knuth, *Advances in Computational mathematics* **5**, 329 (1996).
  - [5] A. Amann, E. Schöll, and W. Just, *Physica A: Statistical Mechanics and its Applications* **373**, 191 (2007).
